# Supplementary material for: Q-MAML: Quantum Model-Agnostic Meta-Learning for Variational Quantum Algorithms
Source: arXiv:2501.05906 source file (2025-01-10)
Supplement: Supplementary file 1 [file 5_appendix.tex]

\subsection{Hamiltonian Task Space} \label{sec:approach}
We define task space of Q-MAML with diverse Hamiltonian, where each Hamiltonian is considered as a single problem to solve in VQE. We handle these probelms in \emph{Hamiltonian Task Space}. In this subsection, we illustrate the definition of \emph{Hamiltonian Task Space} with mathematical and empirical analysis. And we further specify the conditions required for good \emph{Hamiltonian Task Space}.
% \Revise{WRITE SMALL INTRO OF APPROACH} %Now we need to find the /emph{State} in the RL loop on the Quantum side. %Let's define this vector as the Representation Vector.
%\newline % Task Space의 조건 및 정의를 가져와서 힐베르트 공간의 완비성과 코시 수열의 수렴성 직교성, 무한 차원 등으로 논증할 예정
% In this perspective, the Hamiltonian can be thought of as acting as an environment.

%여기까지 개요인데 다듬어야 함
The Hamiltonian is a Hermitian operator that generates the time evolution of a quantum state. In Quantum Computing, the unitary operator $U$ is generated by Hamiltonian. 
\begin{equation}
    U(t)=exp(-\hat{H}t/\hbar)
\end{equation}
First, let's define the \emph{Task Space} of the Hamiltonian.
\begin{definition}[Hamiltonian]
The Hamiltonian operator H is a function defined in a Hilbert space $\mathcal{H}$ as follows:
\begin{equation}
    \hat{H}: \mathcal{H} \rightarrow \mathcal{H}.
\end{equation}
\end{definition}
% \Comment{What is Hamiltonian Task?}
% \Comment{i, n used duplicated times so I used k, m for this definition}
\begin{definition}[Hamiltonian Task Space]
    Let's denote the task space as $\mathcal{T}$. %If the task corresponds to a specific Hamiltonian \Comment{$\hat{H}_m$}, then task space can be defined as a set of Hamiltonians.
    Task space is defined as a set of Hamiltonian.
    \begin{equation}
        \mathcal{T} = \{\hat{H}_1,\hat{H}_2,...,\hat{H}_m\}.
    \end{equation}
\end{definition}
Considering that Hamiltonian serves as a fundamental link between the energy of a system and the quantum state, it is logical to construct task space with a set of Hamiltonian.
%Physically, Hamiltonian has a meaning that connects the energy and quantum state of each physical system, so it is natural to construct a task space with a set of Hamiltonian. \Comment{to jei see comment below}% it is natural 이라는게 물리적인 현상을 만드는게 헤밀토니안 이니까 뭔가 분류되는게? 모이는게 자연스럽다. 그래서 SET을 만든다 라고 녹여내고 싶음

\begin{definition}[Parameterized Hamiltonian Task Space]
When Hamiltonian $\hat{H}$ has representation vector $\phi$, we denote as follows:
%If appropriate $\phi$ can parameterize the Hamiltonian, and the space of its parameters is denoted by $\Phi$. Function $f$ define as follows:%\Revise{We can re-define task space $\mathcal{T}$ with parameterized Hamiltonian as follows:}
    \begin{equation}
    \begin{split}
    f: \Phi \rightarrow \mathcal{T}\\
    f(\phi_m)=\hat{H}_m
    \end{split}
    \end{equation}
\text{where} $\phi \in \Phi$.
\end{definition}

%A good parameterize is one where the distance between parameters is close~\cite{sun2022paco,hausknecht2015deep,ruckstiess2010exploring}, therefore \Revise{if we parameterize Hamiltonian well,} the corresponding Hamiltonian should be close as well. 
% \Comment{PaCo: Parameter-Compositional Multi-task Reinforcement Learning, Parameterized Action Spaces in Deep Reinforcement Learning --> Deep reinforcement learning in parameterized action space?, Exploring Parameter Space in Reinforcement Learning}
\begin{lemma}[The existence of a real-number parameter space]
There is at least one space $\Phi$ in the n-dimensional real-number vector space.
\begin{equation}
    \exists \Phi \subset \mathbf{R}^n
\end{equation}
\end{lemma}
\begin{proof}
    The existence can be demonstrated by considering the eigenvalues of the Hamiltonian as an example. It can be expressed as follows:
    \begin{equation}
        \hat{H} = \sum\limits_n E_i\ket{\psi_i}\bra{\psi_i}
    \end{equation}
    In quantum mechanics, the eigenvector of Hamiltonian forms a basis of Hilbert space. $E_i$ represents energy level and $\ket{\psi_i}$ represents its respect quantum state. Therefore, $E_i$ is a real number and $\ket{\psi_i}$ is a normalized orthogonal eigenvector. % In the eigenvalue problem of Hamiltonian, if the Hamiltonian $\hat{H}$ has n eigenvalues $E_n$, It is expressed as follows.
    % $\hat{H}$ is a self-adjoint operator. Thus, $E_n$ is real value. and $\ket{\psi_n}$ is a normalized orthogonal eigenvector. 
    In general, the Hamiltonian can be decomposed into the product of a unitary matrix $U$ and a diagonal matrix $D$:
    \begin{equation}
    \hat{H} = UDU^\dagger
    \label{eq:udu}
    \end{equation}
    where the diagonal values of $D$ is the eigenvalues of $\hat{H}$, which is real values. Therefore, if we take the diagonal of $D$ as $\phi$, we can define space $\Phi$ that is under real space.
    % \Revise{We define a diagonal vector as the representative vector of Task Space $\mathcal{T}$.}
    \begin{equation}
    \begin{split}
        \text{if}, \phi \equiv diag(D) \newline\\
        \text{then}, \Phi \subset \mathbf{R}^n
    \end{split}
    \label{eq:def}
    \end{equation}
    With~\refeq{def}, we successfully define the parameter space $\Phi$ that satisfies Lemma.
    % Then, We successfully define the parameter space $\Phi$.
\end{proof}

Through linear transformations, infinitely many distinct subspaces can be generated from a given vector space.

\begin{figure}[htbp]
    \centering
     \subfigure[Uniformly Sampled $J_U$]{\includegraphics[width=0.44\columnwidth]{figures/approach_uniform.png} \label{fig:xyz_app_grid}}
     \subfigure[Normally Sampled $J_N$]{\includegraphics[width=0.44\columnwidth]{figures/approach_normal.png} \label{fig:xyz_app_normal}}
    \caption{Relationship between distance in parameter space and task space}
    \label{fig:dimension}
\end{figure}

Using the eigenvalues of the Hamiltonian is an effective method for constructing a representation vector, as it allows us to infer the conditions for a good parameterization.
\begin{conjecture}[Conditions of good parameterizaion]
The good parameterization satisfies the following conditions:
    \begin{enumerate}
        \item Unique Representation\\
        $f$ \text{is injective with respect of} $\phi$
        \begin{equation}
            f(\phi_1) = f(\phi_2), \text{ then } \phi_1 = \phi_2
        \end{equation}
        \item Dimensionality \newline
        Minimize the number of parameters while retaining the model’s ability to adequately describe the Hamiltonian.
        \item Uniform continuity \newline
        Distance function in each space $d_{\Phi}$, $d_{\hat{H}}$ meet the following:
        \begin{equation}
        \begin{split}
            &\text{for every } \phi_1,\phi_2 \in \Phi\\
            &d_{\Phi}(\phi_1,\phi_2) < \sigma ,\text{then } d_{\hat{H}}(\hat{H}_1,\hat{H}_2) < \epsilon
        \end{split}
        \label{eq:conti}
        \end{equation}
    \end{enumerate}
\end{conjecture}
% \begin{example}
Conjectures 5.1 and 5.2 are well-founded, given the definitions of the task space and parameter space, which establish the relevant relationship and constraints. In contrast, the validity of Conjecture 5.3 is less supported by existing data or theoretical results. To show one example that follows Conjecture 5.3, we use a well-known Hamiltonian problem, the Heisenberg XYZ Hamiltonian. 

As we previously explained, Heisenberg XYZ Hamiltonian is defined via three parameters, $J_1$, $J_2$, and $J_3$ and can be obtained by calculating following equation:
% For example as the Heisenberg XYZ Hamiltonian \refeq{heisenberg}   that is defined via three parameters, $J_1$, $J_2$, and $J_3$ as following:
\begin{equation}
    \hat{H}_{XYZ} = - \sum\limits_{n=1}^{N-1} (J_1\sigma^1_n \sigma^1_{n+1} + J_2\sigma^2_n \sigma^2_{n+1} + J_3\sigma^3_n \sigma^3_{n+1})
    \label{eq:heisenberg_append}
\end{equation}
where $\sigma^1, \sigma^2, and \sigma^3$ represent the Pauli X, Y, and Z matrices, respectively.
If we define the distance in Hamiltonian space and parameter space as~\refeq{dist}, we can visualize the relationship between two spaces as in~\reffig{dimension}.
% In this analysis, The distance is defined as \eqref{eq:dist}, the relationship between the two distances can be depicted.
\begin{equation}
\begin{split}
    d_{\hat{H}}(f(\phi_i),f(\phi_j)) \equiv \braket{f(\phi_i)}{f(\phi_j)}\\
    d_{\phi}(\phi_i,\phi_j) \equiv \sum (\phi_i - \phi_j)
\end{split}
\label{eq:dist}
\end{equation}

Figure \ref{fig:xyz_app_grid} showing the parameterization method using $J$ meet the uniform continuity around the point $\hat{H}_{[1,1,1]}$. $J_U$ is sampled from the uniform distribution ($J_U = [J_1, J_2, J_3]$, $J_i \sim \mathcal{U}(-3,5)$). 
Figure \ref{fig:xyz_app_normal} shows that two spaces are linearly correlated around the point $\hat{H}_{[1,1,1]}$. $J_N$ sampled from normal distribution ($J_N = [J_1, J_2, J_3]$, $J_i\sim \mathcal{N}(1,1)$).
According to the results, a good parameterization should satisfy uniform continuity. Specifically, a parameterization based on eigenvectors will be differentiable if and only if the Hamiltonian is differentiable~\cite{smale1967differentiable}.

\subsection{Ansatz for the Experiments}
We utilize different ansatz for problems, where ansatz consisting of IsingXX, IsingYY, and IsingZZ gates is used in the Heisenberg XYZ Hamiltonian (see \reffig{xyz_ansatz}), while StronglyEntanglingLayer is used for molecule Hamiltonian (see \reffig{molecule_ansatz}). It is important to mention that the number of layers in the main text is the same as the number of blocks throughout the circuit.
\begin{figure}[ht]
    \centering
     \subfigure[]{\includegraphics[width=0.7\columnwidth]{figures/xyz_ansatz.png}\label{fig:xyz_ansatz}}
     \subfigure[]{\includegraphics[width=0.7\columnwidth]{figures/mol_ansatz.png}\label{fig:molecule_ansatz}}
     \subfigure[]{\includegraphics[width=0.7\columnwidth]{figures/dist_ansatz.png}\label{fig:dist_ansatz}}
    \caption{(a) Example of ansatz for Heisenberg XYZ Hamiltonian (b) Example of ansatz for molecule Hamiltonian which is named StronglyEntanglingLayer (c) Example of ansatz for distribution embedding, named SimplifiedTwoDesign Layer}
    \label{fig:ansatz}
\end{figure}

\subsection{Molecule Hamiltonian Dataset Generation}
\subsubsection{Parameter Setting}
We select molecules with two symbols to generate molecule Hamiltonian. As some molecules are not able to generate the Hamiltonian with more or less active orbitals, we vary the type of molecule with respect to the active orbitals. \reftab{mol_ham_params_10} and \reftab{mol_ham_params_14} are the parameters we give to the Pennylane function for the Hamiltonian calculation. In both cases, the total amount of data is 60, 12 each per molecule.
\begin{table}[hbt]
\centering
\resizebox{\columnwidth}{!}{
\begin{tabular}{>{\centering\arraybackslash}m{2.5cm} *{5}{>{\centering\arraybackslash}m{1.2cm}}}
\toprule
                                 & $C_2$ & $HF$ & $LiH$ & $Li_2$ & $OH^{-}$ \\ \midrule
Charge                           & 0           & 0         & 0         & 0           & -1           \\
Active Electrons                 & 8           & 8         & 2         & 2           & 8            \\
Bond Length (\AA)                & \multicolumn{5}{c}{0.5, 0.7, 0.9, 1.1, 1.22, 1.3, 1.5, 1.7, 1.9, 2.1, 2.3, 2.5} \\ 
Active Orbitals                  & \multicolumn{5}{c}{5} \\ \bottomrule
\end{tabular}
}
\caption{Parameters for generating 10 qubits molecule Hamiltonian.}
\label{tab:mol_ham_params_10}
\end{table}

\begin{table}[hbt]
\centering
\resizebox{\columnwidth}{!}{
\begin{tabular}{>{\centering\arraybackslash}m{2.5cm} *{5}{>{\centering\arraybackslash}m{1.2cm}}}
\toprule
                                 & $C_2$ & $CO$ & $N_2$ & $Li_2$ & $O_2$ \\ \midrule
Charge                           & 0           & 0         & 0         & 0           & 0           \\
Active Electrons                 & 8           & 10         & 10         & 2           & 12           \\
Bond Length (\AA)                & \multicolumn{5}{c}{0.5, 0.7, 0.9, 1.1, 1.22, 1.3, 1.5, 1.7, 1.9, 2.1, 2.3, 2.5} \\ 
Active Orbitals                  & \multicolumn{5}{c}{7} \\ \bottomrule
\end{tabular}
}
\caption{Parameters for generating 14 qubits molecule Hamiltonian.}
\label{tab:mol_ham_params_14}
\end{table}

\subsection{Heisenberg XYZ Hamiltonian}
In addition to the results provided in the main text, we provide the result of experiments using 10, 14, 16, and 18 qubits (see \reffig{xyz_traj_all}, \reffig{xyz_adap_all}, \reffig{xyz_param_dist_all}, and \reffig{xyz_grad_all}). Overall results well support the explanations we provide in the main text.

\begin{figure*}[ht]
    \centering
     \subfigure[Heisenberg 10 qubits]{\includegraphics[width=0.31\textwidth]{figures/xyz_10qubit_train_epoch_loss_perf_fin.png} }
         \subfigure[Heisenberg 12 qubits]{\includegraphics[width=0.31\textwidth]{figures/xyz_12qubit_train_epoch_loss_perf_fin.png} }
     \subfigure[Heisenberg 14 qubits]{\includegraphics[width=0.31\textwidth]{figures/xyz_14qubit_train_epoch_loss_perf_fin.png} }
         \subfigure[Heisenberg 16 qubits]{\includegraphics[width=0.31\textwidth]{figures/xyz_16qubit_train_epoch_loss_perf_fin.png} }
         \subfigure[Heisenberg 18 qubits]{\includegraphics[width=0.31\textwidth]{figures/xyz_18qubit_train_epoch_loss_perf_fin.png} }
         \subfigure[Heisenberg 20 qubits]{\includegraphics[width=0.31\textwidth]{figures/xyz_20qubit_train_epoch_loss_perf_fin.png} }
    \caption{Training trajectory of \emph{Leaner} with Heisenberg XYZ dataset.}
    \label{fig:xyz_traj_all}
\end{figure*}

\begin{figure*}[ht]
    \centering
     \subfigure[Heisenberg 10 qubits]{\includegraphics[width=0.31\textwidth]{figures/xyz_10_ham_gap_0.05_sigma_test_error_fin.png} }
         \subfigure[Heisenberg 12 qubits]{\includegraphics[width=0.31\textwidth]{figures/xyz_12_ham_gap_0.05_sigma_test_error_fin.png} }
     \subfigure[Heisenberg 14 qubits]{\includegraphics[width=0.31\textwidth]{figures/xyz_14_ham_gap_0.05_sigma_test_error_fin.png} }
         \subfigure[Heisenberg 16 qubits]{\includegraphics[width=0.31\textwidth]{figures/xyz_16_ham_gap_0.05_sigma_test_error_fin.png} }
         \subfigure[Heisenberg 18 qubits]{\includegraphics[width=0.31\textwidth]{figures/xyz_18_ham_gap_0.05_sigma_test_error_fin.png} }
         \subfigure[Heisenberg 20 qubits]{\includegraphics[width=0.31\textwidth]{figures/xyz_20_ham_gap_0.05_sigma_test_error_fin.png} }
    \caption{Training trajectory of PQC in adaptation phase with Heisenberg XYZ dataset.}
    \label{fig:xyz_adap_all}
\end{figure*}

\begin{figure*}[ht]
    \centering
     \subfigure[Heisenberg 10 qubits]{\includegraphics[width=0.31\textwidth]{figures/xyz_10qubit_distance_distribution_fin.png} }
         \subfigure[Heisenberg 12 qubits]{\includegraphics[width=0.31\textwidth]{figures/xyz_12qubit_distance_distribution_fin.png} }
     \subfigure[Heisenberg 14 qubits]{\includegraphics[width=0.31\textwidth]{figures/xyz_14qubit_distance_distribution_fin.png} }
         \subfigure[Heisenberg 16 qubits]{\includegraphics[width=0.31\textwidth]{figures/xyz_16qubit_distance_distribution_fin.png} }
         \subfigure[Heisenberg 18 qubits]{\includegraphics[width=0.31\textwidth]{figures/xyz_18qubit_distance_distribution_fin.png} }
         \subfigure[Heisenberg 20 qubits]{\includegraphics[width=0.31\textwidth]{figures/xyz_20qubit_distance_distribution_fin.png} }
    \caption{Statistics of the parameter initialized using Q-MAML, Uniform, and Gaussian on Heisenberg XYZ Hamiltonian dataset.}
    \label{fig:xyz_param_dist_all}
\end{figure*}

\begin{figure*}[ht]
    \centering
     \subfigure[Heisenberg 10 qubits]{\includegraphics[width=0.31\textwidth]{figures/xyz_grad_10qubit_circuit_grad_fin.png} }
         \subfigure[Heisenberg 12 qubits]{\includegraphics[width=0.31\textwidth]{figures/xyz_grad_12qubit_circuit_grad_fin.png} }
     \subfigure[Heisenberg 14 qubits]{\includegraphics[width=0.31\textwidth]{figures/xyz_grad_14qubit_circuit_grad_fin.png} }
         \subfigure[Heisenberg 16 qubits]{\includegraphics[width=0.31\textwidth]{figures/xyz_grad_16qubit_circuit_grad_fin.png} }
         \subfigure[Heisenberg 18 qubits]{\includegraphics[width=0.31\textwidth]{figures/xyz_grad_18qubit_circuit_grad_fin.png} }
         \subfigure[Heisenberg 20 qubits]{\includegraphics[width=0.31\textwidth]{figures/xyz_grad_20qubit_circuit_grad_fin.png} }
    \caption{Trend of the PQC's gradient norm during pre-training phase with Heisenberg XYZ Hamiltonian dataset.}
    \label{fig:xyz_grad_all}
\end{figure*}

\begin{figure*}[ht]
    \centering
     \subfigure[Heisenberg 10 qubits]{\includegraphics[width=0.31\textwidth]{figures/xyz_vqa_grad_10qubit_fin.png} }
     \subfigure[Heisenberg 12 qubits]{\includegraphics[width=0.31\textwidth]{figures/xyz_vqa_grad_12qubit_fin.png} }
     \subfigure[Heisenberg 14 qubits]{\includegraphics[width=0.31\textwidth]{figures/xyz_vqa_grad_14qubit_fin.png} }
     \subfigure[Heisenberg 16 qubits]{\includegraphics[width=0.31\textwidth]{figures/xyz_vqa_grad_16qubit_fin.png} }
     \subfigure[Heisenberg 18 qubits]{\includegraphics[width=0.31\textwidth]{figures/xyz_vqa_grad_18qubit_fin.png} }
     \subfigure[Heisenberg 20 qubits]{\includegraphics[width=0.31\textwidth]{figures/xyz_vqa_grad_20qubit_fin.png} }
    \caption{Fluctuation of gradient norm of PQC while training in the adaptation phase.}
    \label{fig:xyz_vqa_all}
\end{figure*}

\subsection{Molecule Hamiltonian}
For the readability of the figures, we additionally provide the enlarged version of figures of Molecule Hamiltonian experiments provided in the main text. \emph{We should note that the result of \reffig{molecule_10_adap} is slightly updated for Gaussian as \reffig{molecule_10_adap} the data used to plot the figure is result of parameters sampled from $\mathcal{N}(0,1)$, while the correct value with $\frac{1}{360}$ is used for \reffig{large_adap_mol_edit}.}

\begin{figure*}[hbt!]
    \centering
     \subfigure[Molecule 10 qubits]{\includegraphics[width=0.9\columnwidth]{figures/mol_10qubit_train_epoch_loss_perf_fin.png} }
     \subfigure[Molecule 14 qubits]{\includegraphics[width=0.9\columnwidth]{figures/mol_14qubit_train_epoch_loss_perf_fin.png} }
    \caption{Enlarged version of training trajectory of \emph{Learner} with Molecule Hamiltonian.}
    \label{fig:large_learner_mol}
\end{figure*}

\begin{figure*}
    \centering
     \subfigure[Molecule 10 qubits]{\includegraphics[width=0.9\columnwidth]{figures/molecule_10_ham_gap_validaiton_variance_0.05_sigma_test_fin_c.png}\label{fig:large_adap_mol_edit} }
     \subfigure[Molecule 14 qubits]{\includegraphics[width=0.9\columnwidth]{figures/molecule_14_ham_gap_validaiton_variance_0.05_sigma_test_fin.png} }
    \caption{Enlarged version of training trajectory of PQC in the adaptation phase. The average gap value is plotted using 6 different Molecule Hamiltonian. The shaded regions indicate one standard deviation ($[\mu-\sigma/2, \mu+\sigma/2]$).}
    \label{fig:large_pqc_mol}
\end{figure*}

\begin{figure*}[ht]
    \centering
     \subfigure[Molecule 10 qubits]{\includegraphics[width=0.9\columnwidth]{figures/molecule_10qubit_distance_distribution_sigma_fin.png}}
     \subfigure[Molecule 14 qubits]{\includegraphics[width=0.9\columnwidth]{figures/molecule_14qubit_distance_distribution_sigma_fin.png} }
    \caption{Statistics of the parameter initialized using Q-MAML, Uniform, and Gaussian.}
    \label{fig:large_gen_stat_mol}
\end{figure*}

\begin{figure*}[ht]
    \centering
     \subfigure[Molecule 10 qubits]{\includegraphics[width=0.9\columnwidth]{figures/mol_grad_10qubit_circuit_grad_fin.png}}
         \subfigure[Molecule 14 qubits]{\includegraphics[width=0.9\columnwidth]{figures/mol_grad_14qubit_circuit_grad_fin.png}}
    \caption{Trend of the PQC's gradient norm during pre-training phase}
    \label{fig:large_grad_curve_mol}
\end{figure*}

\begin{figure*}[ht]
    \centering
     \subfigure[Molecule 10 qubits]{\includegraphics[width=0.9\columnwidth]{figures/mol_vqa_grad_10qubit_fin.png}}
         \subfigure[Molecule 14 qubits]{\includegraphics[width=0.9\columnwidth]{figures/mol_vqa_grad_14qubit_fin.png}}
    \caption{Fluctuation of gradient norm of PQC while training in the adaptation phase.}
    \label{fig:large_vqa_grad_mol}
\end{figure*}

\subsection{Distribution Embedding}

In this experiment, we aim to show the efficiency of proposed framework by using common task of quantum computing. Amplitude embedding is crucial in quantum computing when dealing with classical data. %Unlike other experiments, we use classical loss functions such as L2 and KLDloss.%, and still suffers from the exponential amount of gates required when the number of qubit increases. 
The most popular amplitude embedding method is proposed by~\citet{mottonen2004transformation}, which requires numerous gates and exponential depth required as the number of qubits increases. However, as we described in \reftab{amp_gate}, our Q-MAML can achieve acceptable performance with comparatively few gate usage. We further show the performance of Q-MAML by providing fast adaptation on diverse distributions.

\begin{table}[!hbt]
\centering
\resizebox{\columnwidth}{!}{
\begin{tabular}{lcccccc}
\toprule
                    & \multicolumn{6 }{c}{\# of Qubits} \\ 
                    & 4   & 5   & 6   & 7   & 8   & 9   \\ \midrule
Amplitude Embedding & 29    & 61    & 125    & 253    & 509    & 1021   \\
Q-MAML (2 layers)   & 22    & 29    & 36    & 43    &  50   &  57  \\
Q-MAML (4 layers)   & 40    & 53    & 66    & 79    & 92    & 105   \\ \bottomrule
\end{tabular}
}
\caption{The number of gates used to conduct amplitude embedding and for Q-MAML on PQC with 2 layers and 4 layers per number of qubits.}
\label{tab:amp_gate}
\end{table}

\subsubsection{Task Space Definition}
The target vector of dimension $2^{qubit}$ is defined as the target vector and is used as a task space. Each distribution is considered a task in this problem.
% \begin{equation}
%     \mathcal{T} = \{T_i: T_i = Y_{true} \subset \mathcal{R}^n \}
% \end{equation}
\subsubsection{Dataset Generation}
We generate different distributions using three kinds of distribution functions: Random distribution, %Gaussian distribution, 
and Log-normal distribution. Random distribution is generated by measuring the output of PQC with random initialization. We use 5 layers of SimplifiedTwoDesign~\cite{cerezo2021cost} to generate Random distributions, and a total 10000 number of samples are generated. 
For Log-normal distribution, various $\mu$ and $\sigma$ values are used to generate various shapes of distribution.
% For Gaussian distribution and Log-normal distribution, \ReviseB{various $\mu$ and $\sigma$ value is used to generate diverse shape of distribution.}
%each data point is composed with 10,000,000 random sampled values from Log-normal or Normal distribution with various $\mu$ and $\sigma$ value to generate diverse shape of distribution function. 
For $\mu$, we use values $\{0.5, 0.75, 1.0, 1.25, 1.50, 1.75, 2.0, 2.25, 2.5, 2.75, 3.0\}$, and for $\sigma$, $\{0.5, 0.75, 1.0, 1.25, 1.5, 1.75, 2.0\}$ is used. An example of a log-normal distribution data set is provided in~\reffig{dist_example}.
% \Comment{More Clear for lognormal and normal}

\subsubsection{Experiment Design}
For the \emph{Learner} architecture, everything is the same as other experiments except the input layer of the \emph{Learner} varies by the number of qubits. With $n$ number of qubits, the input size will be defined as $2^n$. For PQC, the 4 repeats of SimplifedTwoDesign~\cite{cerezo2021cost} layers are used, with 4, 7, and 9 %4, 5, 6, 7, 8, 9, and 10 
qubits. The most different point in this experiment is not aimed at solving the Hamiltonian problem, the cost function is Kulback-Leibler (KL) divergence to compare the output of Q-MAML and the target distribution. 
Furthermore, \emph{Learner} is trained on Random distribution, and the adaptation performance is measured using 16 randomly sampled %Gaussian or 
Log-normal distributions. In the adaptation phase, a single PQC is trained to embed a single distribution.

\begin{figure*}[ht]
    \centering
     \subfigure[Log-normal 4 qubits]{\includegraphics[width=0.31\textwidth]{figures/lognormal_viz_4.png} }
     % \subfigure[Random 5 qubits]{\includegraphics[width=0.31\textwidth]{figures/5_train_loss.png} }
     % \subfigure[\Comment{Random 6 qubits}]{\includegraphics[width=0.31\textwidth]{figures/4_train_loss.png} }
     \subfigure[Log-normal 7 qubits]{\includegraphics[width=0.31\textwidth]{figures/lognormal_viz_7.png} }
     % \subfigure[\Comment{Random 8 qubits}]{\includegraphics[width=0.31\textwidth]{figures/4_train_loss.png} }
     \subfigure[Log-normal 9 qubits]{\includegraphics[width=0.31\textwidth]{figures/lognormal_viz_9.png} }
     % \subfigure[\Comment{Random 10 qubits}]{\includegraphics[width=0.31\textwidth]{figures/4_train_loss.png} }
    \caption{Example of target distribution embedding}
    \label{fig:dist_example}
\end{figure*}

\begin{figure*}[ht]
    \centering
     \subfigure[Random 4 qubits]{\includegraphics[width=0.31\textwidth]{figures/4_train_loss.png} }
     % \subfigure[Random 5 qubits]{\includegraphics[width=0.31\textwidth]{figures/5_train_loss.png} }
     % \subfigure[\Comment{Random 6 qubits}]{\includegraphics[width=0.31\textwidth]{figures/4_train_loss.png} }
     \subfigure[Random 7 qubits]{\includegraphics[width=0.31\textwidth]{figures/7_train_loss.png} }
     % \subfigure[\Comment{Random 8 qubits}]{\includegraphics[width=0.31\textwidth]{figures/4_train_loss.png} }
     \subfigure[Random 9 qubits]{\includegraphics[width=0.31\textwidth]{figures/9_train_loss.png} }
     % \subfigure[\Comment{Random 10 qubits}]{\includegraphics[width=0.31\textwidth]{figures/4_train_loss.png} }
    \caption{Training trajectory of \emph{Leaner} trained with random distribution dataset.}
    \label{fig:dist_train_traj}
\end{figure*}

\begin{figure*}
    \centering
     \subfigure[Log-normal 4 qubits]{\includegraphics[width=0.31\textwidth]{figures/dist_grad_4qubit_circuit_grad_fin.png} }
     % \subfigure[Log-normal 5 qubits]{\includegraphics[width=0.31\textwidth]{figures/5_train_loss.png} }
     % \subfigure[\Comment{Log-normal 6 qubits}]{\includegraphics[width=0.31\textwidth]{figures/4_train_loss.png} }
     \subfigure[Log-normal 7 qubits]{\includegraphics[width=0.30\textwidth]{figures/dist_grad_7qubit_circuit_grad_fin.png} }
     % \subfigure[\Comment{Log-normal 8 qubits}]{\includegraphics[width=0.31\textwidth]{figures/4_train_loss.png} }
     \subfigure[Log-normal 9 qubits]{\includegraphics[width=0.32\textwidth]{figures/dist_grad_9qubit_circuit_grad_fin.png} }
     % \subfigure[\Comment{Log-normal 10 qubits}]{\includegraphics[width=0.31\textwidth]{figures/4_train_loss.png} }
    \caption{Trend of the PQC's gradient norm during the pre-training phase.}
    \label{fig:dist_grad_learner}
\end{figure*}

\begin{figure*}
    \centering
     \subfigure[Log-normal 4 qubits]{\includegraphics[width=0.30\textwidth]{figures/dist_4_pqc_loss_fin_cut.png} }
     % \subfigure[Log-normal 5 qubits]{\includegraphics[width=0.31\textwidth]{figures/5_train_loss.png} }
     % \subfigure[\Comment{Log-normal 6 qubits}]{\includegraphics[width=0.31\textwidth]{figures/4_train_loss.png} }
     \subfigure[Log-normal 7 qubits]{\includegraphics[width=0.31\textwidth]{figures/dist_7_pqc_loss_fin_cut.png} }
     % \subfigure[\Comment{Log-normal 8 qubits}]{\includegraphics[width=0.31\textwidth]{figures/4_train_loss.png} }
     \subfigure[Log-normal 9 qubits]{\includegraphics[width=0.32\textwidth]{figures/dist_9_pqc_loss_fin_cut.png} }
     % \subfigure[\Comment{Log-normal 10 qubits}]{\includegraphics[width=0.31\textwidth]{figures/4_train_loss.png} }
    \caption{Training trajectory of PQC with Log-normal distribution. 16 different distributions are randomly sampled and trained on different PQC to measure the average loss. The shaded regions indicate one standard deviation ($[\mu-\sigma/2, \mu+\sigma/2]$).}
    \label{fig:dist_adap_log}
\end{figure*}

\begin{figure*}
    \centering
     \subfigure[Log-normal 4 qubits]{\includegraphics[width=0.31\textwidth]{figures/dist_4_pqc_gradd_loss_fin_cut.png} }
     % \subfigure[Log-normal 5 qubits]{\includegraphics[width=0.31\textwidth]{figures/5_train_loss.png} }
     % \subfigure[\Comment{Log-normal 6 qubits}]{\includegraphics[width=0.31\textwidth]{figures/4_train_loss.png} }
     \subfigure[Log-normal 7 qubits]{\includegraphics[width=0.31\textwidth]{figures/dist_7_pqc_gradd_loss_fin_cut.png} }
     % \subfigure[\Comment{Log-normal 8 qubits}]{\includegraphics[width=0.31\textwidth]{figures/4_train_loss.png} }
     \subfigure[Log-normal 9 qubits]{\includegraphics[width=0.31\textwidth]{figures/dist_9_pqc_gradd_loss_fin_cut.png} }
     % \subfigure[\Comment{Log-normal 10 qubits}]{\includegraphics[width=0.31\textwidth]{figures/4_train_loss.png} }
    \caption{Fluctuation of gradient norm of PQC while training in the adaptation phase.}
    \label{fig:dist_adap_grad}
\end{figure*}

\begin{figure*}
    \centering
     \subfigure[1 Iteration 4 qubits]{\includegraphics[width=0.30\textwidth]{figures/4_gen_at_0.png} }
     \subfigure[100 Iteration 4 qubits]{\includegraphics[width=0.31\textwidth]{figures/4_gen_at_99.png} }
     \subfigure[1000 Iteration 4 qubits]{\includegraphics[width=0.32\textwidth]{figures/4_gen_at_999.png} }
     \subfigure[1 Iteration 7 qubits]{\includegraphics[width=0.30\textwidth]{figures/7_gen_at_0.png} }
     \subfigure[100 Iteration 7 qubits]{\includegraphics[width=0.31\textwidth]{figures/7_gen_at_99.png} }
     \subfigure[1000 Iteration 7 qubits]{\includegraphics[width=0.32\textwidth]{figures/7_gen_at_999.png} }
     \subfigure[1 Iteration 9 qubits]{\includegraphics[width=0.30\textwidth]{figures/9_gen_at_0.png} }
     \subfigure[100 Iteration 9 qubits]{\includegraphics[width=0.31\textwidth]{figures/9_gen_at_99.png} }
     \subfigure[1000 Iteration 9 qubits]{\includegraphics[width=0.32\textwidth]{figures/9_gen_at_999.png} }
    \caption{Result of distribution embedding with the Log-normal dataset with different qubits and iteration.}
    \label{fig:dist_adap_vis}
\end{figure*}

\begin{figure*}
    \centering
     \subfigure[Random 4 qubits]{\includegraphics[width=0.31\textwidth]{figures/dist_4qubit_distance_distribution_sigma_fin.png} }
     % \subfigure[Log-normal 5 qubits]{\includegraphics[width=0.31\textwidth]{figures/5_train_loss.png} }
     % \subfigure[\Comment{Log-normal 6 qubits}]{\includegraphics[width=0.31\textwidth]{figures/4_train_loss.png} }
     \subfigure[Random 7 qubits]{\includegraphics[width=0.31\textwidth]{figures/dist_7qubit_distance_distribution_sigma_fin.png} }
     % \subfigure[\Comment{Log-normal 8 qubits}]{\includegraphics[width=0.31\textwidth]{figures/4_train_loss.png} }
     \subfigure[Random 9 qubits]{\includegraphics[width=0.31\textwidth]{figures/dist_9qubit_distance_distribution_sigma_fin.png} }
     % \subfigure[\Comment{Log-normal 10 qubits}]{\includegraphics[width=0.31\textwidth]{figures/4_train_loss.png} }
    \caption{Statistics of the parameter initialized using Q-MAML, Uniform, and Gaussian. For each qubit, the optimal pretrained learner was used to infer a random dataset. The pretraining was conducted with a random dataset.}
    \label{fig:dist_param_stat}
\end{figure*}

\begin{figure*}
    \centering
     \subfigure[Log-normal 4 qubits]{\includegraphics[width=0.31\textwidth]{figures/lognormal_dist_4qubit_distance_distribution_sigma_fin.png} }
     % \subfigure[Log-normal 5 qubits]{\includegraphics[width=0.31\textwidth]{figures/5_train_loss.png} }
     % \subfigure[\Comment{Log-normal 6 qubits}]{\includegraphics[width=0.31\textwidth]{figures/4_train_loss.png} }
     \subfigure[Log-normal 7 qubits]{\includegraphics[width=0.30\textwidth]{figures/lognormal_dist_7qubit_distance_distribution_sigma_fin.png} }
     % \subfigure[\Comment{Log-normal 8 qubits}]{\includegraphics[width=0.31\textwidth]{figures/4_train_loss.png} }
     \subfigure[Log-normal 9 qubits]{\includegraphics[width=0.31\textwidth]{figures/lognormal_dist_9qubit_distance_distribution_sigma_fin.png} }
     % \subfigure[\Comment{Log-normal 10 qubits}]{\includegraphics[width=0.31\textwidth]{figures/4_train_loss.png} }
    \caption{Statistics of the parameter initialized using Q-MAML, Uniform, and Gaussian. For each qubit, the optimal pretrained learner was used to infer a log-normal dataset. The pretraining was conducted with a random dataset.}
    \label{fig:dist_log_param_stat}
\end{figure*}

% \begin{figure*}
%     \centering
%      \subfigure[Log-normal 4 qubits]{\includegraphics[width=0.31\textwidth]{figures/dist_4_pqc_gradd_loss_fin_cut.png} }
%      % \subfigure[Log-normal 5 qubits]{\includegraphics[width=0.31\textwidth]{figures/5_train_loss.png} }
%      % \subfigure[\Comment{Log-normal 6 qubits}]{\includegraphics[width=0.31\textwidth]{figures/4_train_loss.png} }
%      \subfigure[Log-normal 7 qubits]{\includegraphics[width=0.31\textwidth]{figures/dist_7_pqc_gradd_loss_fin_cut.png} }
%      % \subfigure[\Comment{Log-normal 8 qubits}]{\includegraphics[width=0.31\textwidth]{figures/4_train_loss.png} }
%      \subfigure[Log-normal 9 qubits]{\includegraphics[width=0.31\textwidth]{figures/dist_9_pqc_gradd_loss_fin_cut.png} }
%      % \subfigure[\Comment{Log-normal 10 qubits}]{\includegraphics[width=0.31\textwidth]{figures/4_train_loss.png} }
%     \caption{Fluctuation of gradient norm of PQC while training in the adaptation phase.}
%     \label{fig:dist_adap_grad}
% \end{figure*}

\subsubsection{Results}

\reffig{dist_train_traj} shows the training trajectory of \emph{Learner}. We select the parameter of \emph{Learner} when the loss value is minimum for the adaptation phase. For the 4-qubit experiment, the \emph{Learner} trained for 3 epochs is selected, while for 7 qubits epoch 26, and 9 qubits epoch 30. The $\gamma^2$ for Gaussian initialization is set to $\frac{1}{168}$.
In~\reffig{dist_adap_log}, we visualize the adaptation performance in the log-normal dataset. As we can see from the figure, Q-MAML overall converges well on the log-normal dataset concerning the number of qubits. We analyze the statistics of the output of \emph{Learner} in~\reffig{dist_param_stat} and~\reffig{dist_log_param_stat}, where even though the identical \emph{Learner} is used to generate values between the random distribution and the log-normal distribution, it shows distinctive patterns. Furthermore, when the number of qubits increases, this pattern still holds, which implies that our Q-MAML can make \emph{Learner} learn the characteristics of the task despite the number of qubits.

In a 4-qubit environment, overfit is observed. We think the 4-qubit environment is too simple compared to our \emph{Learner} design which causes fitting issues. However, as the number of qubits increases, the complexity also rises, which helps mitigate this issue (see~\reffig{dist_train_traj}). The size of the dataset and the structure of the classical model are kept constant to ensure a fair evaluation. Additionally, the Gradient Norm shows a similar trend, further supporting this observation (see~\reffig{dist_grad_learner}). %This result implies that we can leverage the optimization knowledge we have accumulated through classical machine learning.
We visualize the embedding result in~\reffig{dist_adap_vis}, where PQC at iteration 1, 100, and 500 is selected per qubits. The results are selected as random rather than being hand-picked.

Furthermore, Q-MAML is both effective and broadly applicable to most Quantum Machine Learning techniques that use a classical loss function as a cost function.
% Moreover, this method is both effective and broadly applicable to most QML techniques that use a cost function as a classical loss function.

% In~\reffig{dist_vqe_traj}, the training trajectory on 16 different distributions is shown. For the \emph{Learner}, we use the same \emph{Learner} selected in the Pre-training phase which trained on Random distribution, and for the PQC it is aimed to fit either Log-normal distribution or Normal distribution. 
